# Supplementary material for: STaDA: Style Transfer as Data Augmentation
Source: arXiv:1909.01056 source file (2019-09-03)
Supplement: Supplementary file 1 [file appendix1.tex]

\chapter{Image Styles}
\begin{figure}[!ht]
\begin{subfigure}{.22\textwidth}
  \centering
  \includegraphics[width=\linewidth]{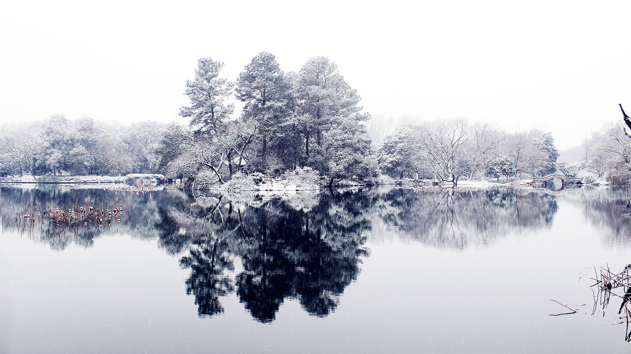}
  \caption{A Snow picture, simple but beautiful}
\end{subfigure}
\begin{subfigure}{.22\textwidth}
  \centering
  \includegraphics[width=\linewidth]{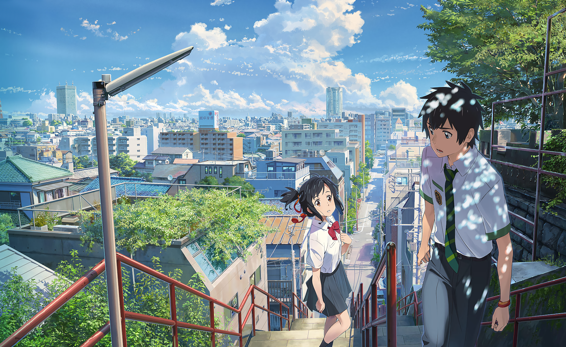}
  \caption{Japaness Animation: Your Name (2016)}
\end{subfigure}
\begin{subfigure}{.22\textwidth}
  \centering
  \includegraphics[width=\linewidth]{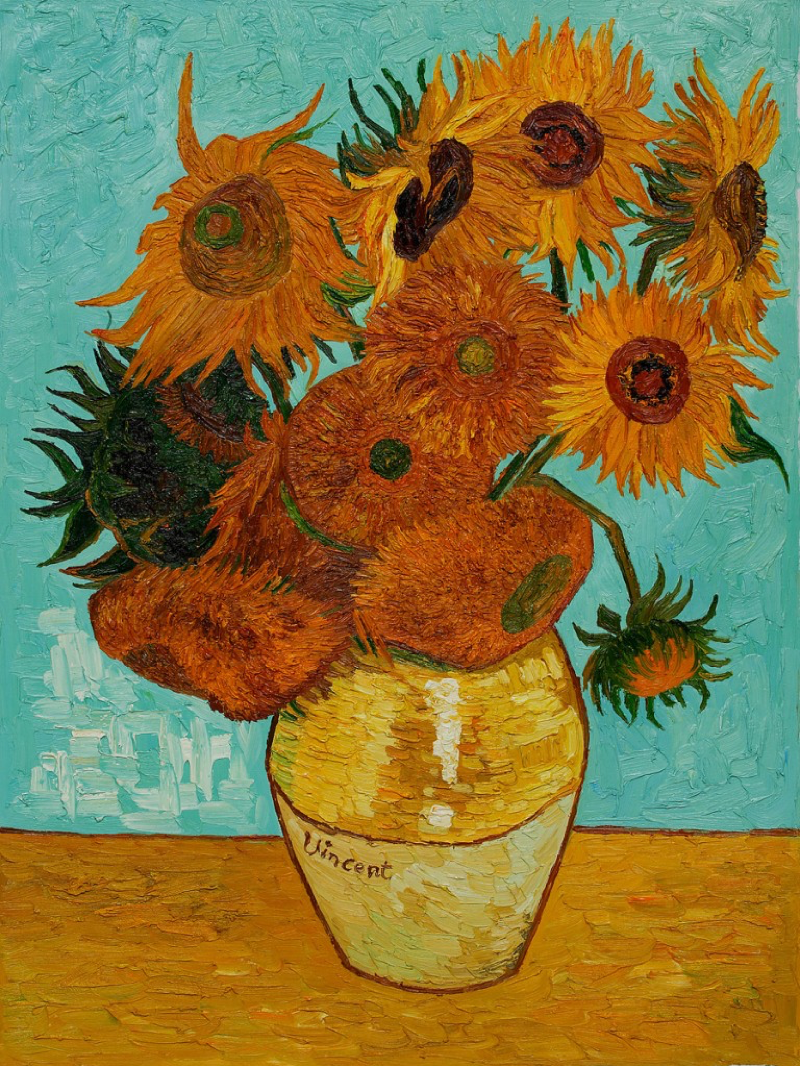}
  \caption{Sunflower from one of Van Gogh's series of paintings}
\end{subfigure}
\begin{subfigure}{.22\textwidth}
  \centering
  \includegraphics[width=\linewidth]{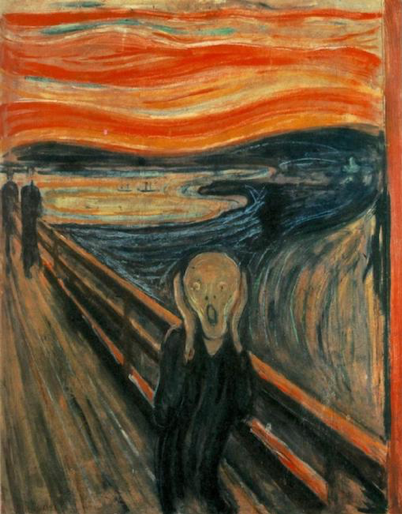}
  \caption{The Scream, Edvard Munch, 1893 - 1910}
\end{subfigure}
\begin{subfigure}{.22\textwidth}
  \centering
  \includegraphics[width=\linewidth]{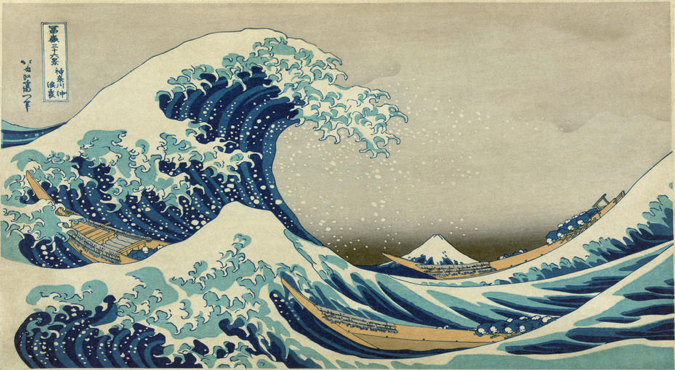}
  \caption{The Great Wave off Kanagawa, Hokusai, 1829 - 1832}
\end{subfigure}
\begin{subfigure}{.22\textwidth}
  \centering
  \includegraphics[width=\linewidth]{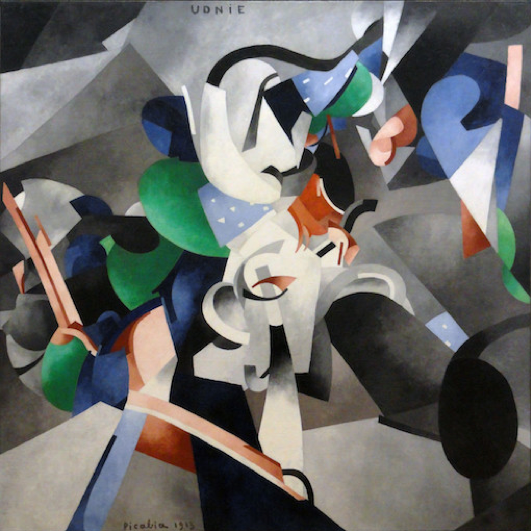}
  \caption{A typical udnie painting \newline}
\end{subfigure}
\begin{subfigure}{.22\textwidth}
  \centering
  \includegraphics[width=\linewidth]{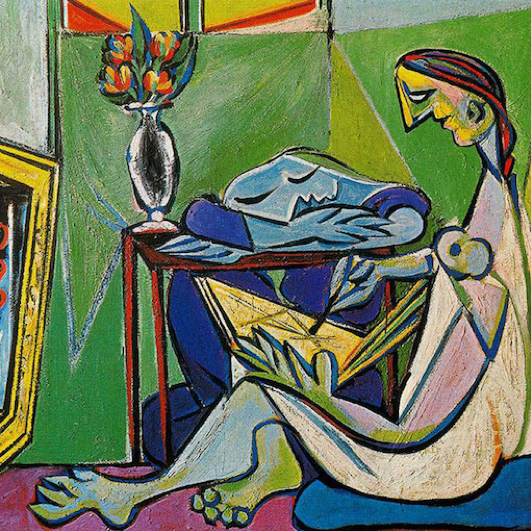}
  \caption{The Muse, Pablo Picasso, 1935}
\end{subfigure}
\hspace{2ex}
\begin{subfigure}{.22\textwidth}
  \centering
  \includegraphics[width=\linewidth]{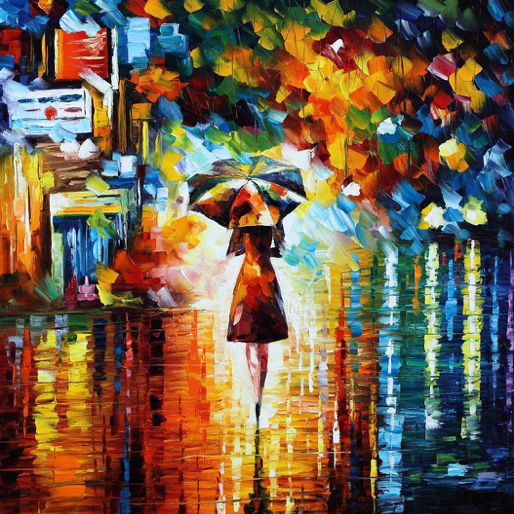}
  \caption{Rain Princess, a painting by Leonid Afremov}
\end{subfigure}
\caption{Eight Styles}
\end{figure}
