# Supplementary material for: STaDA: Style Transfer as Data Augmentation
Source: arXiv:1909.01056 source file (2019-09-03)
Supplement: Supplementary file 3 [file appendix2.tex]

\chapter{GitHub Link}
The entire implementation code can be found on GitHub: \url{https://github.com/zhengxu001/neural-data-augmentation}.
